# Supplementary material for: Predictive and Generative Neural Networks for Object Functionality
Source: arXiv:2006.15520 source file (2020-06-28)
Supplement: Supplementary file 1 [file appendix.tex]

\appendix
\section{Subnetwork architectures}
\label{sec:architecture}
